# Supplementary material for: Demystifying Video Reasoning
Source: arXiv:2603.16870 source file (2026-07-31)
Supplement: Supplementary file 2 [file distilled_example_arxiv.tex]

% \begin{figure}[!h]
% \centering
% \includegraphics[width=\textwidth]{figures/supp/distilled_example1.pdf}

% \includegraphics[width=\textwidth]{figures/supp/distilled_example2.pdf}
% \caption{Qualitative visualizations of the distilled model.}
% \end{figure}

\begin{figure}[!b]
\centering
\includegraphics[width=\textwidth]{figures/supp/distilled_example1_arxiv.pdf}
\caption{Qualitative visualizations of distilled model.}
\end{figure}
\begin{figure}[!t]\ContinuedFloat
\centering
\includegraphics[width=\textwidth]{figures/supp/distilled_example1_arxiv_continued.pdf}
\end{figure} 

\begin{figure}[!t]\ContinuedFloat
\centering
\includegraphics[width=\textwidth]{figures/supp/distilled_example2.pdf}
\caption{(continued) Qualitative visualizations of distilled model.}
\end{figure}
