# Supplementary material for: Demystifying Video Reasoning
Source: arXiv:2603.16870 source file (2026-07-31)
Supplement: Supplementary file 4 [file wan21.tex]

\begin{figure}[!h]
\vspace{-8pt}
\centering
\includegraphics[width=\textwidth]{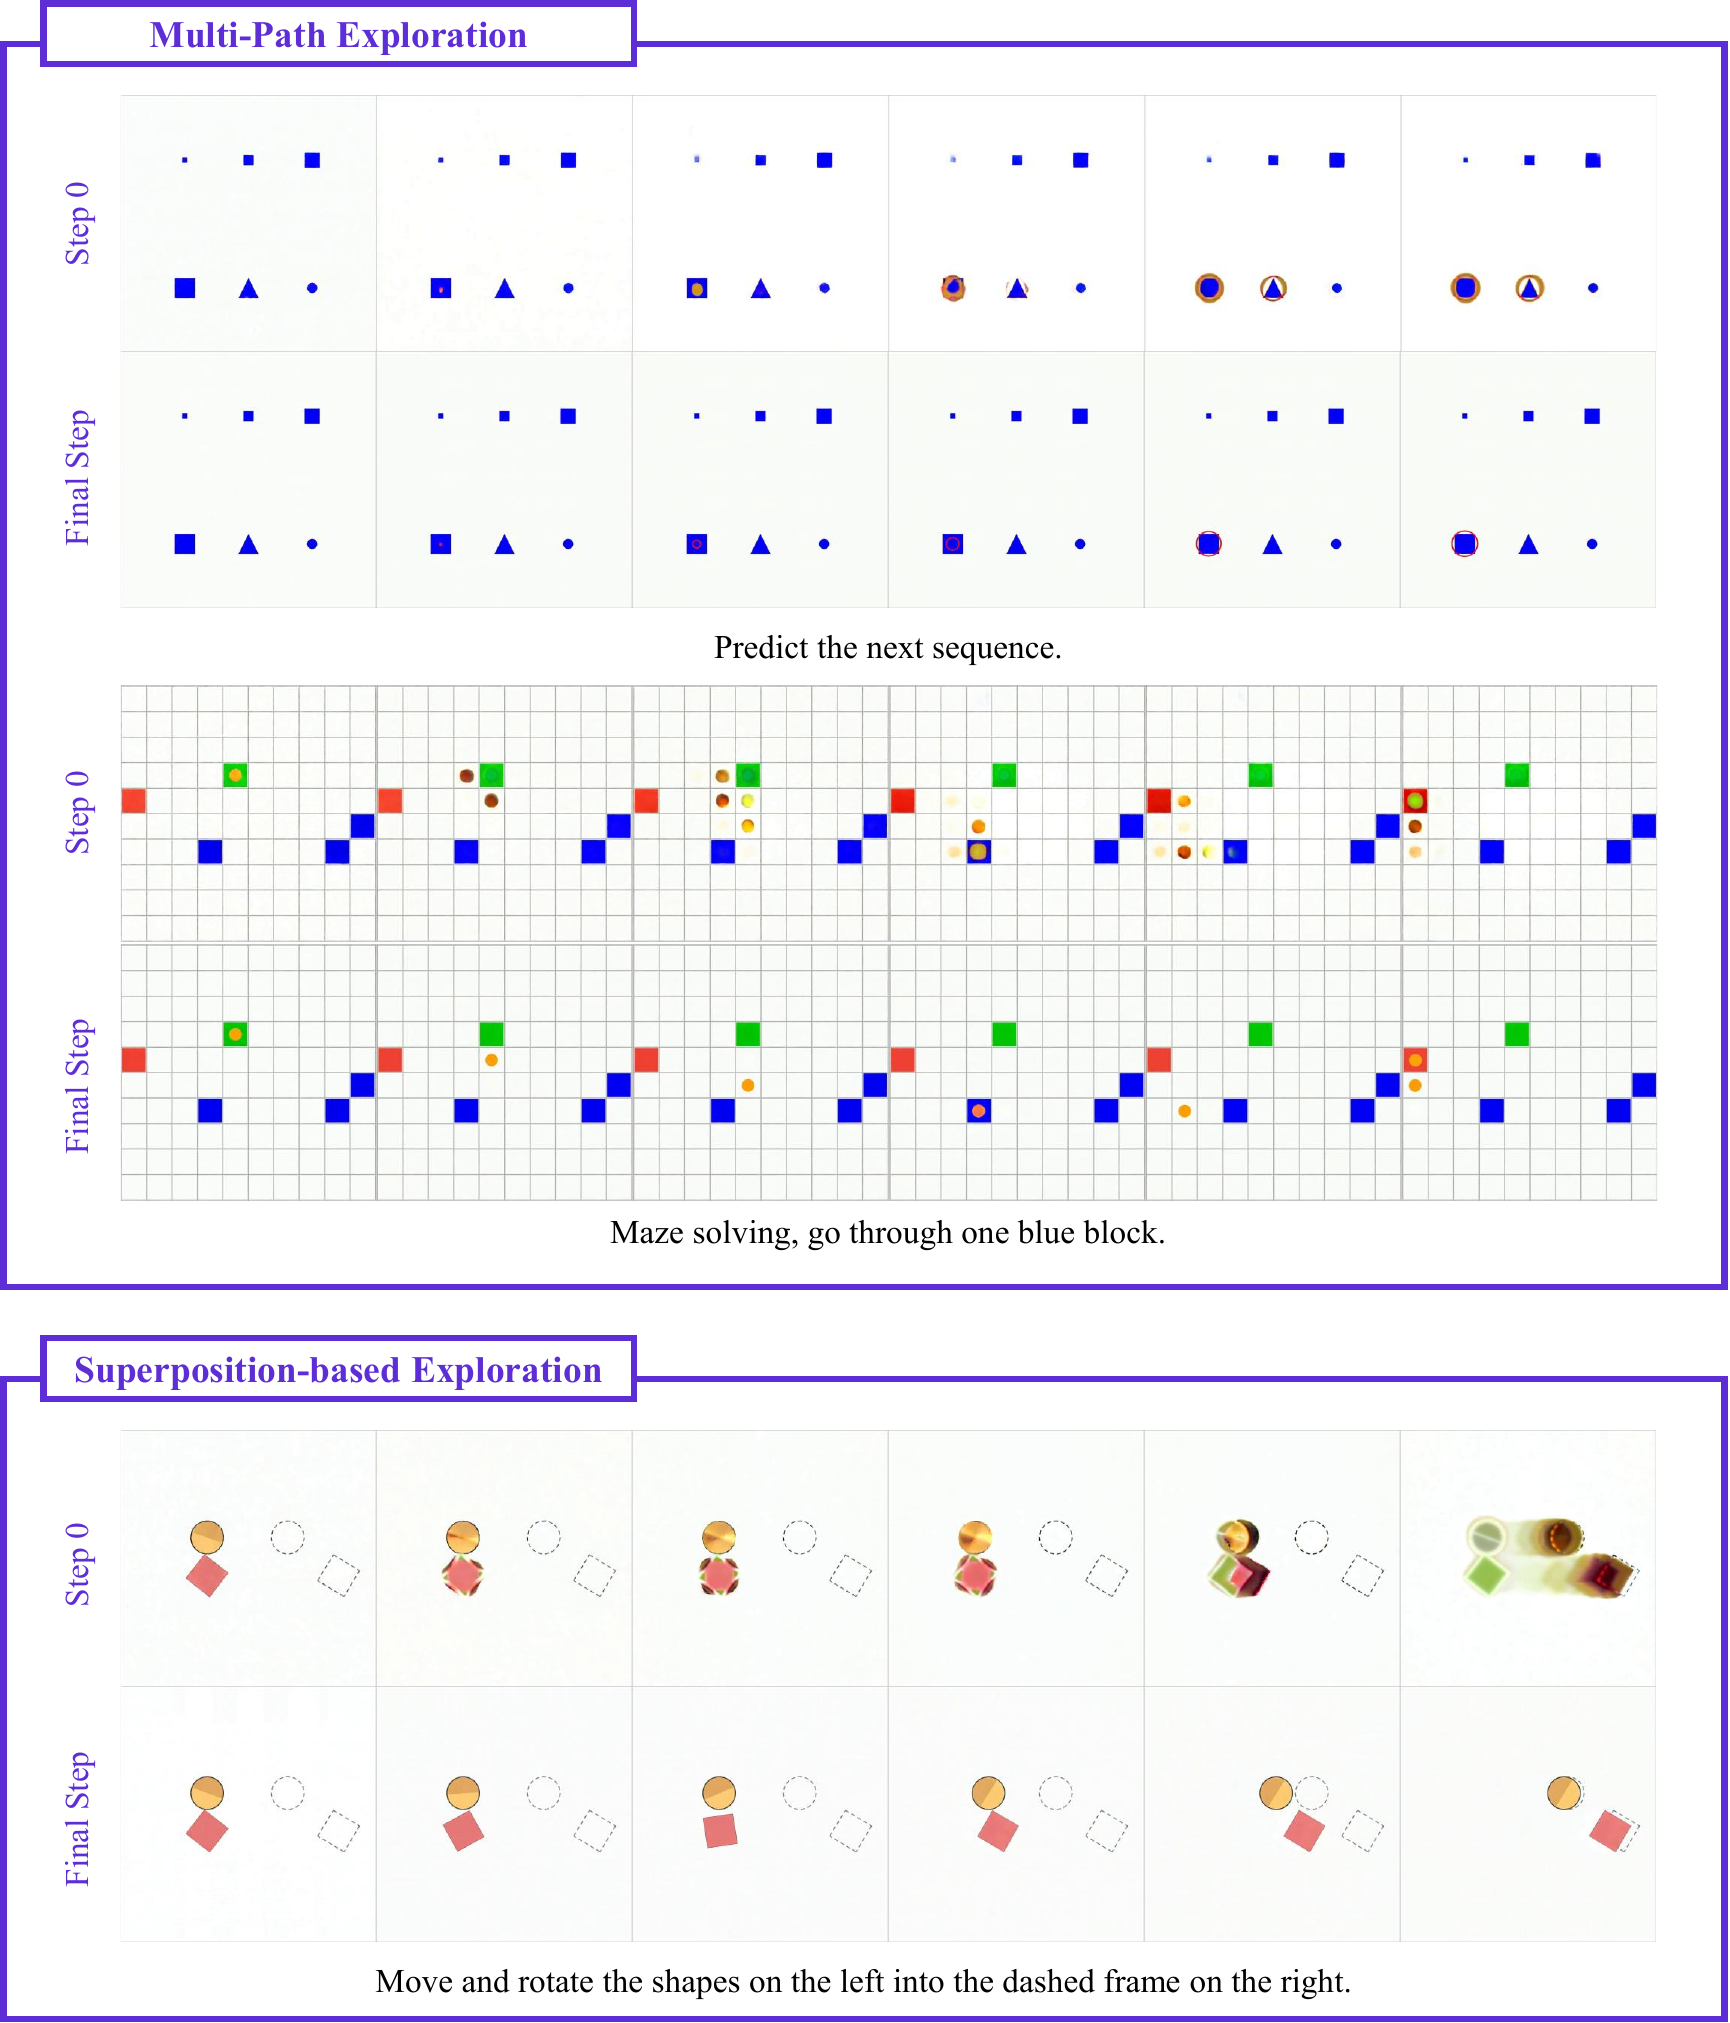}
\caption{Qualitative examples on VBVR-Wan2.1.}
\label{fig:viz_wan21}
\end{figure}

\begin{figure}[!h]\ContinuedFloat
\centering
\includegraphics[width=\textwidth]{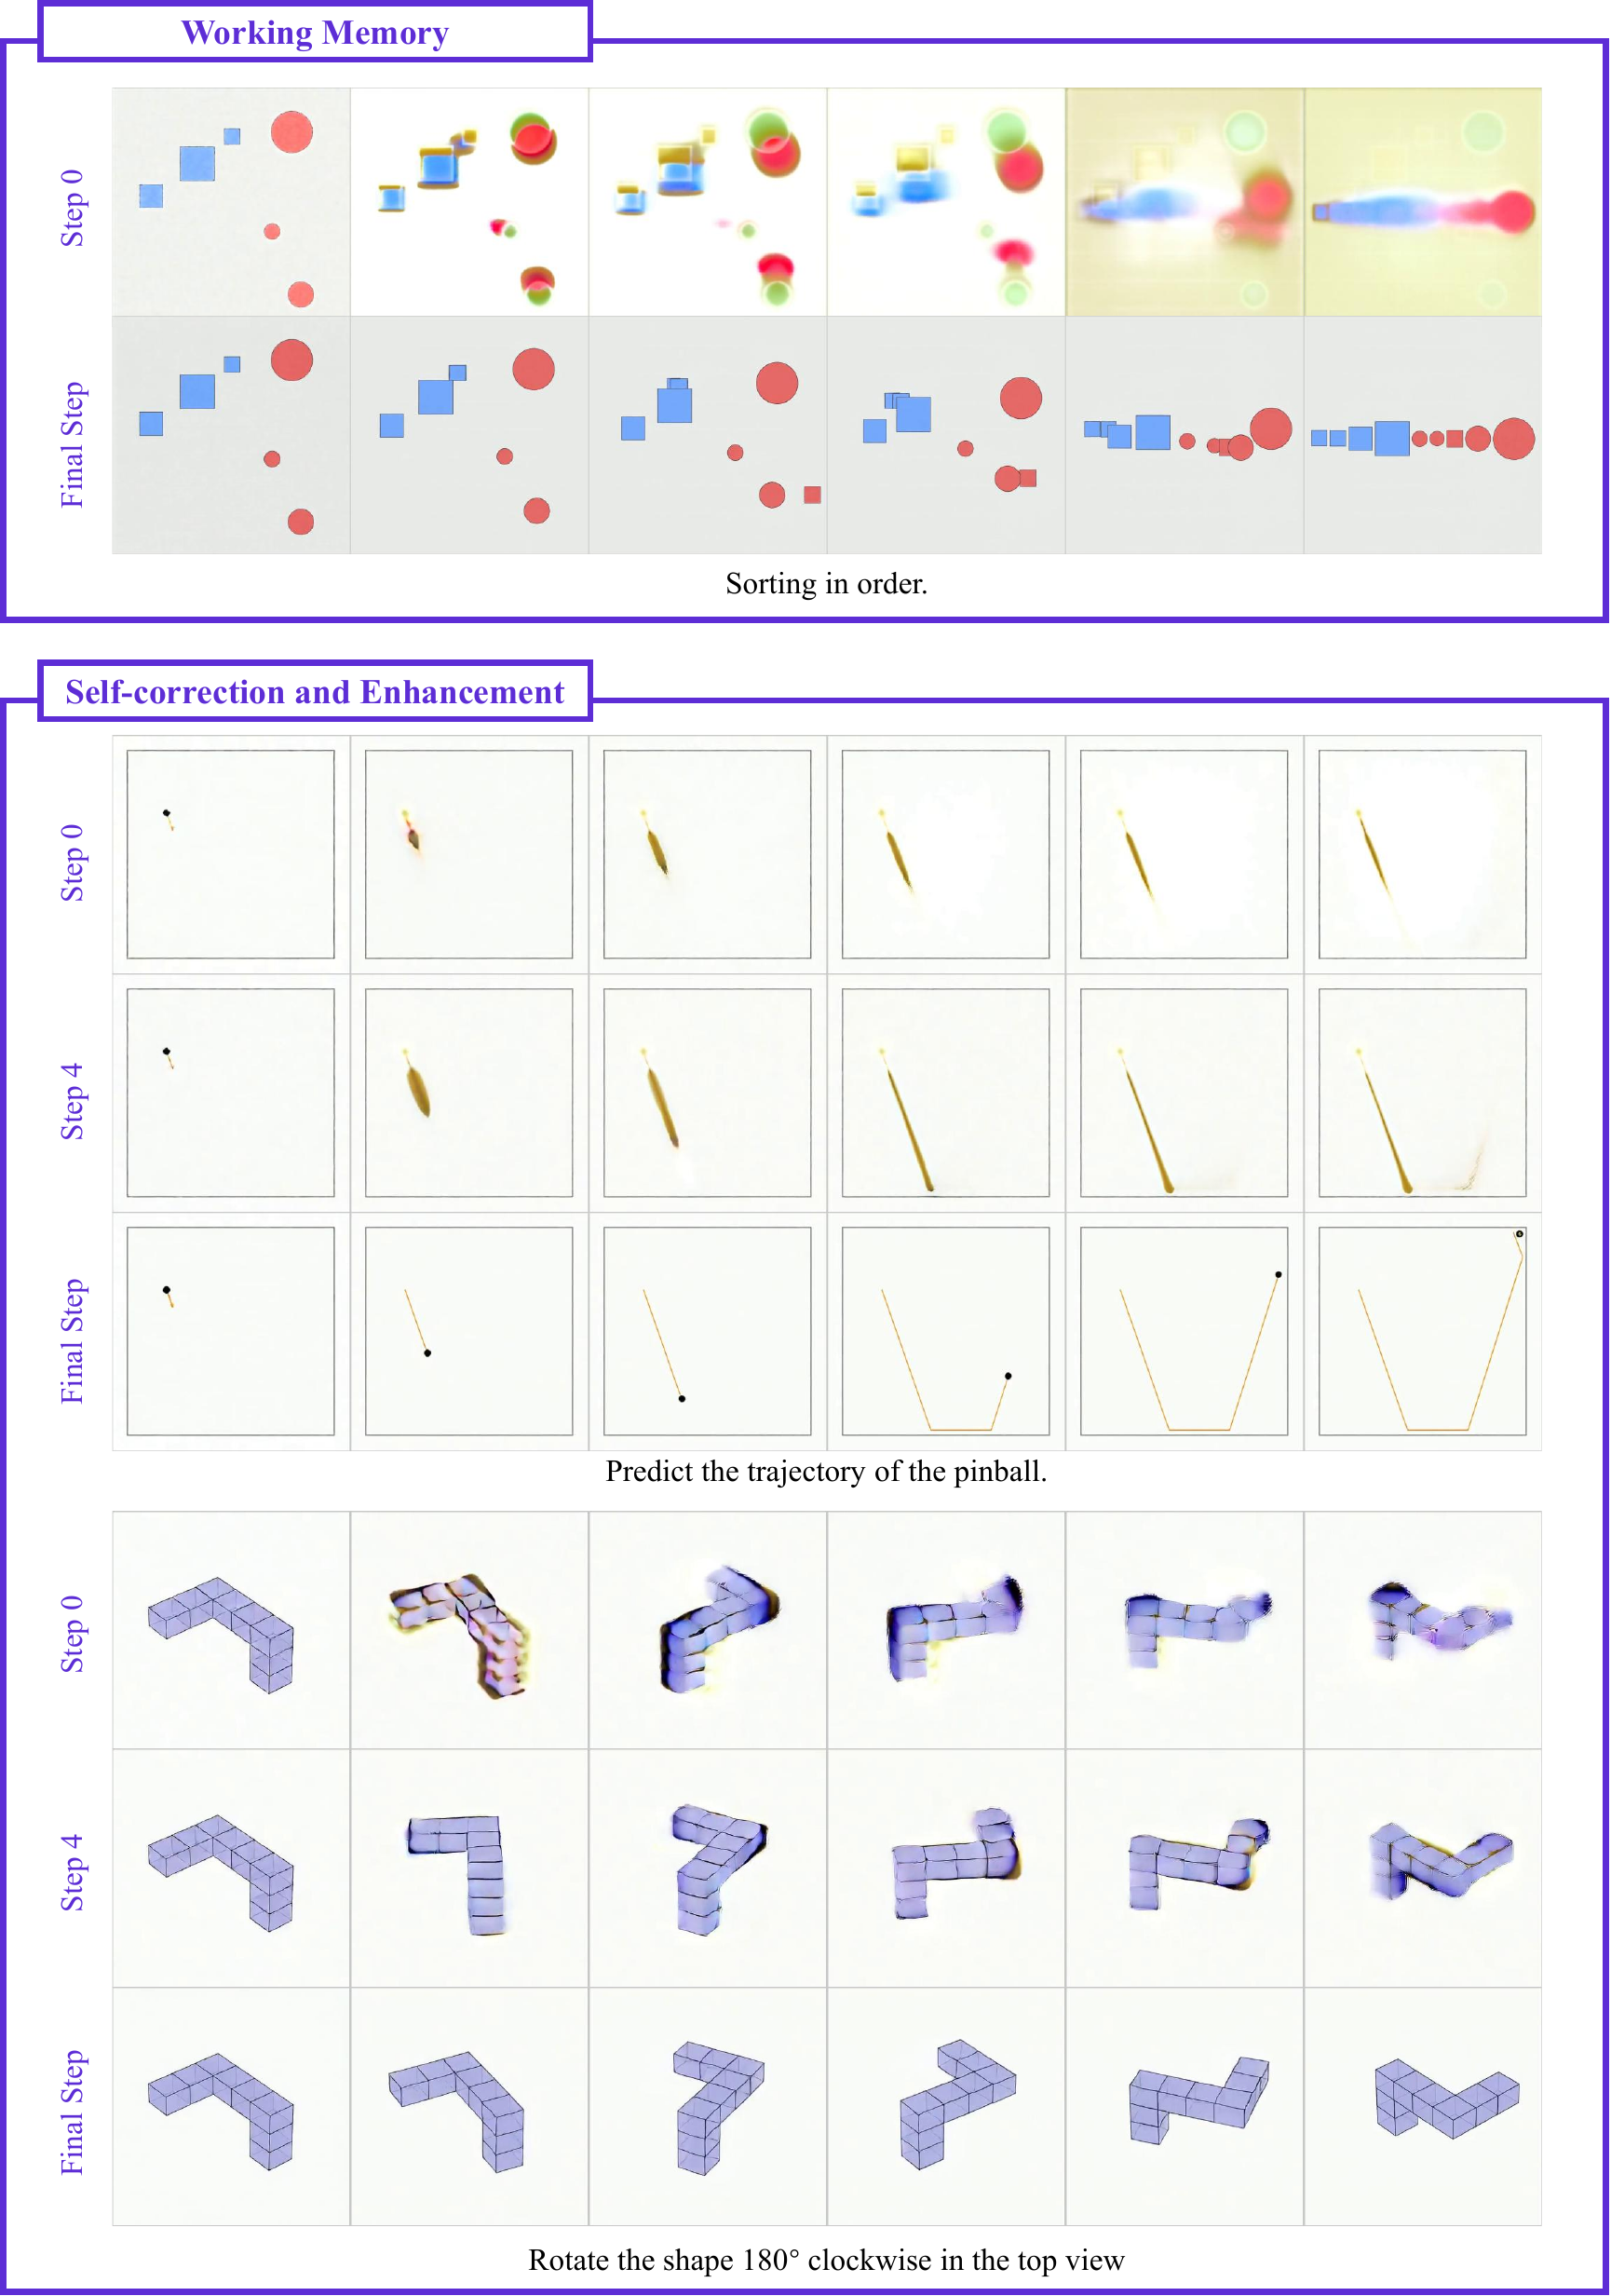}
\caption{(Continued) Qualitative examples on VBVR-Wan2.1.}
\end{figure}
